# Supplementary material for: Quantifying protocols for safe school activities
Source: arXiv:2204.07148 source file (2022-04-13)
Supplement: Supplementary file 6 [file canada_schools.tex]

\chapter{Canada schools}
\label{sec:canada_schools}

{\color{red} TO BE REMOVED: their model differs from ours, and a straight comparison cannot be made. For the purpose of justifying the $p_m$ values we used, it suffices to reference one of their tables}
