# Supplementary material for: Quantifying protocols for safe school activities
Source: arXiv:2204.07148 source file (2022-04-13)
Supplement: Supplementary file 7 [file closed_schools_baseline.tex]

\chapter{Closed schools as baseline}
\label{sec:closed_schools_baseline}
