# Supplementary material for: Quantifying protocols for safe school activities
Source: arXiv:2204.07148 source file (2022-04-13)
Supplement: Supplementary file 8 [file networks_social_dynamics.tex]

\chapter{Network social dynamics}
\label{sec:network_social_dynamics}
